# Supplementary material for: Mapping electron beam-induced radiolytic damage in molecular crystals
Source: arXiv:2404.18011 source file (2024-04-27)
Supplement: Supplementary file 1 [file damage_SI.pdf]

## Materials and Methods

### Materials

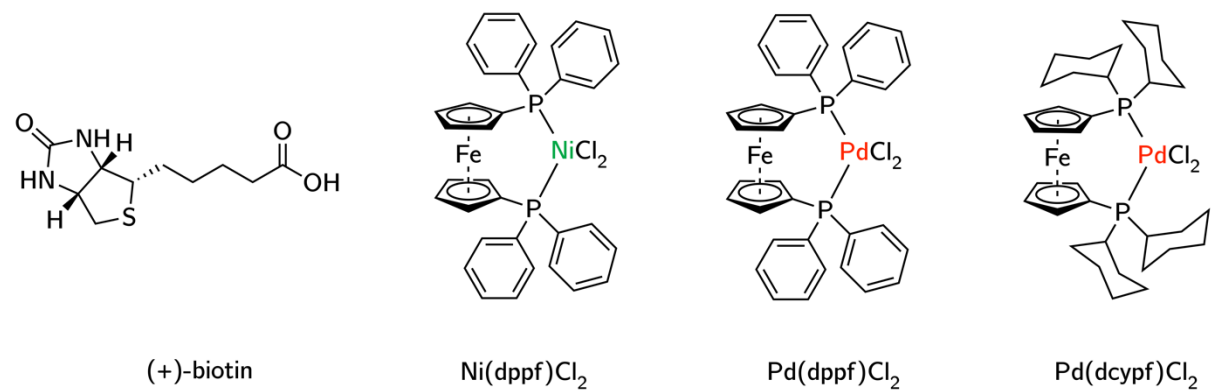

**Fig. S1.** Schematics of (+)-biotin, Ni(dppf)Cl<sub>2</sub>, Pd(dppf)Cl<sub>2</sub>, and Pd(dcyfp)Cl<sub>2</sub>. Abbreviations: dppf = 1,1'-bis(diphenylphosphino)ferrocene, dcyfp = 1,1'-bis(dicyclohexylphosphino)ferrocene.

(+)-Biotin (Sigma-Aldrich; CAS No. 58-85-5) is a visibly microcrystalline white to off-white powder. Since the distribution of well-diffracting nanocrystals by simple shake-n-bake was subpar, (+)-biotin was recrystallized by dissolving 10 mg in 5 mL boiling nanopure deionized water and allowing the resultant colorless solution to gradually cool to RT. Showers of high-quality, colorless single crystals precipitated after 10 minutes; the resultant suspension was diluted 10× with ethanol and dropcast onto lacey carbon 300 mesh Au grids (Ted Pella; Product No. 01895G).

Ni(dppf)Cl<sub>2</sub> (Sigma-Aldrich; CAS No. 67292-34-6) is a visibly microcrystalline, dark green iridescent powder. 10 mg of this compound was crushed between siliconized glass coverslips and gently applied to lacey carbon 300 mesh Au grids (Ted Pella; Product No. 01895G).

Pd(dppf)Cl<sub>2</sub> (Sigma-Aldrich; CAS No. 72287-26-4) is a visibly microcrystalline, dark orange iridescent powder. 10 mg of this compound was crushed between siliconized glass coverslips and gently applied to lacey carbon 300 mesh Au grids (Ted Pella; Product No. 01895G).

Pd(dcyfp)Cl<sub>2</sub> (Sigma-Aldrich; CAS No. 917511-90-1) is a visibly microcrystalline, dull reddish-orange powder. 10 mg of this compound was crushed between siliconized glass coverslips and gently applied to lacey carbon 300 mesh Au grids (Ted Pella; Product No. 01895G).

## Methods: 4D-STEM

All scanning nanobeam electron diffraction experiments were conducted at an accelerating voltage of 200 or 300 kV on the double-aberration-corrected TEAM 0.5 instrument located at the National Center for Electron Microscopy facility of the Molecular Foundry at Lawrence Berkeley National Laboratory. Before data acquisition, the incident beam current was reduced to the detection threshold of the fluorescent screen ammeter ( $<40$  pA) by using the monochromator focus as a continuously adjustable gun lens. Beam flux was estimated from previous reference measurements using a Faraday cup and an ammeter under similar conditions. A near-parallel probe was formed by using a custom  $10\text{ }\mu\text{m}$  C2 aperture (Norcada) to access a range of narrow ( $<0.1$  mrad) semiconvergence angles. Using a custom DigitalMicrograph script, multiscan 4D-STEM data were acquired with the 4D Camera operating at 87000 frames per second. As an illustrative example, each biotin dataset is comprised of  $512\times 512$  probe positions and  $576\times 576$  detector pixels, resulting in 174 GB of raw data per scan. These raw data were counted and reduced to a sparse, linear-index-encoded electron event representation (EER) in HDF5 format on the NERSC supercomputer, Perlmutter, using the open-source software package [stempy](#). All data are publicly available on [Zenodo](#). HDF5 files can be interactively viewed using the open-source software package [DuSC explorer](#).

|                                      |                                    |
|--------------------------------------|------------------------------------|
| Accelerating voltage                 | 300 kV                             |
| Semiconvergence angle                | 0.07 mrad                          |
| Scan dimensions                      | $512\times 512$                    |
| Real-space step size                 | 9.22 nm                            |
| Estimated probe size (FWHM)          | 14.4 nm                            |
| Total illuminated area               | $11.2\text{ }\mu\text{m}^2$        |
| Estimated fluence per probe position | $0.15\text{ e}^- \text{ \AA}^{-2}$ |
| Total size of raw data               | 4350 GB                            |
| Total size of sparsified data        | 2.18 GB                            |

**Table S1.** Experimental parameters for 4D-STEM scans on biotin.

|                                      |                                   |
|--------------------------------------|-----------------------------------|
| Accelerating voltage                 | 200 kV                            |
| Semiconvergence angle                | 0.07 mrad                         |
| Scan dimensions                      | $256\times 256$                   |
| Real-space step size                 | 15.1 nm                           |
| Estimated probe size (FWHM)          | 18.4 nm                           |
| Total illuminated area               | $7.5\text{ }\mu\text{m}^2$        |
| Estimated fluence per probe position | $1.5\text{ e}^- \text{ \AA}^{-2}$ |
| Total size of raw data               | 13200 GB                          |
| Total size of sparsified data        | 9.93 GB                           |

**Table S2.** Experimental parameters for 4D-STEM scans on  $\text{Ni(dppf)Cl}_2$ .

### Methods: 3D ED

All 3D ED experiments were conducted at an accelerating voltage of 300 kV on an FEI Tecnai F30 transmission electron microscope equipped with a TVIPS TemCam-XF416 camera. Generally, the workflow for 3D ED involved the dispersion of a nanocrystalline powder onto a lacey carbon grid, subsequent insertion of the grid into the TEM, and then a prolonged search to find well-diffracting samples. After a suitable single crystal was identified, usually in overfocused diffraction (i.e., shadow imaging) mode, a 1  $\mu\text{m}$  post-specimen selected area aperture was inserted to isolate the specimen of interest. Next, the crystal was exposed to parallel illumination and unidirectionally rotated at an angular speed of 0.3 degrees per second. During this process, a series of diffraction patterns were continuously acquired using 3-second exposures throughout the angular wedge sampled. Data were converted to SMV format and processed using XDS [40].

## Supplementary Text

### Appendix A: Nomenclature

In this work, we chose to use the term “coherently diffracting zone” (CDZ) to describe self-consistent areas of the real-space lattice that produce monolithic diffraction patterns. We note that some precedent for this term exists in the mineralogy literature [41], [42]. In some cases, these CDZs resemble classical phenomena known as bend contours [43], [44], in which continuous deformation of a perfect lattice leads to narrow, lance-like, curved fringes of diffraction contrast. For instance, some CDZs in our biotin dataset (Fig. 1D-F) correspond well to shapes observed in studies of classical bend contours, which have historically been well-characterized in thin (tens of nm) crystalline foils easily susceptible to forcible mechanical bending. Nevertheless, we also observed a range of CDZs whose morphologies diverge significantly from the typical appearance of bend contours (Fig. 3, S4-S5), suggesting a distinct origin. Furthermore, the thicknesses of the crystals interrogated in our 4D-STEM measurements (estimated at 200-300 nm, hundreds of unit cells thick) significantly exceed the thicknesses of thin foils (<50 nm, tens of unit cells thick) typically linked with bend contours, and it is unclear whether simple bending adequately accounts for the diverse and often unpredictable range of CDZ shapes we have observed.

We intend “coherently diffracting zone” to function as a more general term. A CDZ corresponds to any area within the real-space lattice which diffracts self-consistently enough to produce the same set of Bragg reflections over some arbitrary length scale (identifiable by placing reciprocal-space virtual apertures around these peaks and reconstructing virtual dark-field images). Intrinsic heterogeneity in the distribution of CDZs does not necessarily have to conform to mosaicity induced by sample bending, and in many cases the shapes and morphologies of CDZs appear rotationally misoriented and discontinuous. We view bend contours as a specific subset of CDZs which obey certain constraints (i.e. induced by smooth, continuous deformation or bending). Choice of syntax aside, the rearrangement of CDZs (including bend contours) due to electron beam-induced radiolysis is phenomenologically very relevant to 3D

electron crystallography, where current data processing routines simply do not account for these effects.

## Appendix B: Spectroscopic corroboration

Recognizing that diffraction alone cannot provide a complete picture of the chemical effects of radiolytic damage, we set out to briefly investigate whether electron energy-loss spectroscopy (EELS) could serve as a parallel metric for assessing beam-induced chemical destruction in these systems. In particular, aromaticity is known to produce an EELS resonance at an energy loss of approximately 6 eV [15], corresponding to the same  $\pi$ - $\pi^*$  electronic transition typically probed by ultraviolet-visible spectroscopy.

We used parallel-beam TEM to record both EEL spectra and selected-area electron diffraction (SAED) patterns from the same crystal of dppf (Fig. S8). After the initial acquisition of an EEL spectrum from an individual nanocrystal, each specimen was continuously irradiated until the corresponding SAED patterns had completely faded. Subsequent acquisition of another EEL spectrum (Fig. S9) revealed that the 6 eV peak remained intact, confirming that crystallographic destruction precedes chemical destruction in these species. We note that the dispersion of this peak is fairly broad, and superior energy resolution would likely split this signal into several subsidiary maxima representing the different energy levels of the  $\pi$ - $\pi^*$  transitions in the cyclopentadienyl (Cp) rings versus the phenyl (Ph) rings. Chemical interpretation is premature at this stage, but future work will interrogate whether the signal for the negatively charged Cp rings decays at a different rate compared to the neutral Ph rings.

Furthermore, our EEL spectra indicate that a typical inelastic collision during an electron diffraction experiment involves an energy loss of approximately 22 eV (Fig. S10). To contextualize, this value is 4-5 $\times$  higher than the homolytic bond dissociation enthalpy of an average  $sp^3$  C—F bond (4-5 eV), generally considered one of the strongest bonds in

organic chemistry [45]. Although it is unclear whether this progression of events will hold in nonaromatic compounds, we note that the recent development of monochromated STEM beams with sub-10 meV resolution in the infrared regime [46] provides an excellent range of spectroscopic handles (e.g., the decay of a C—H stretching mode) for assessing this in greater chemical detail.

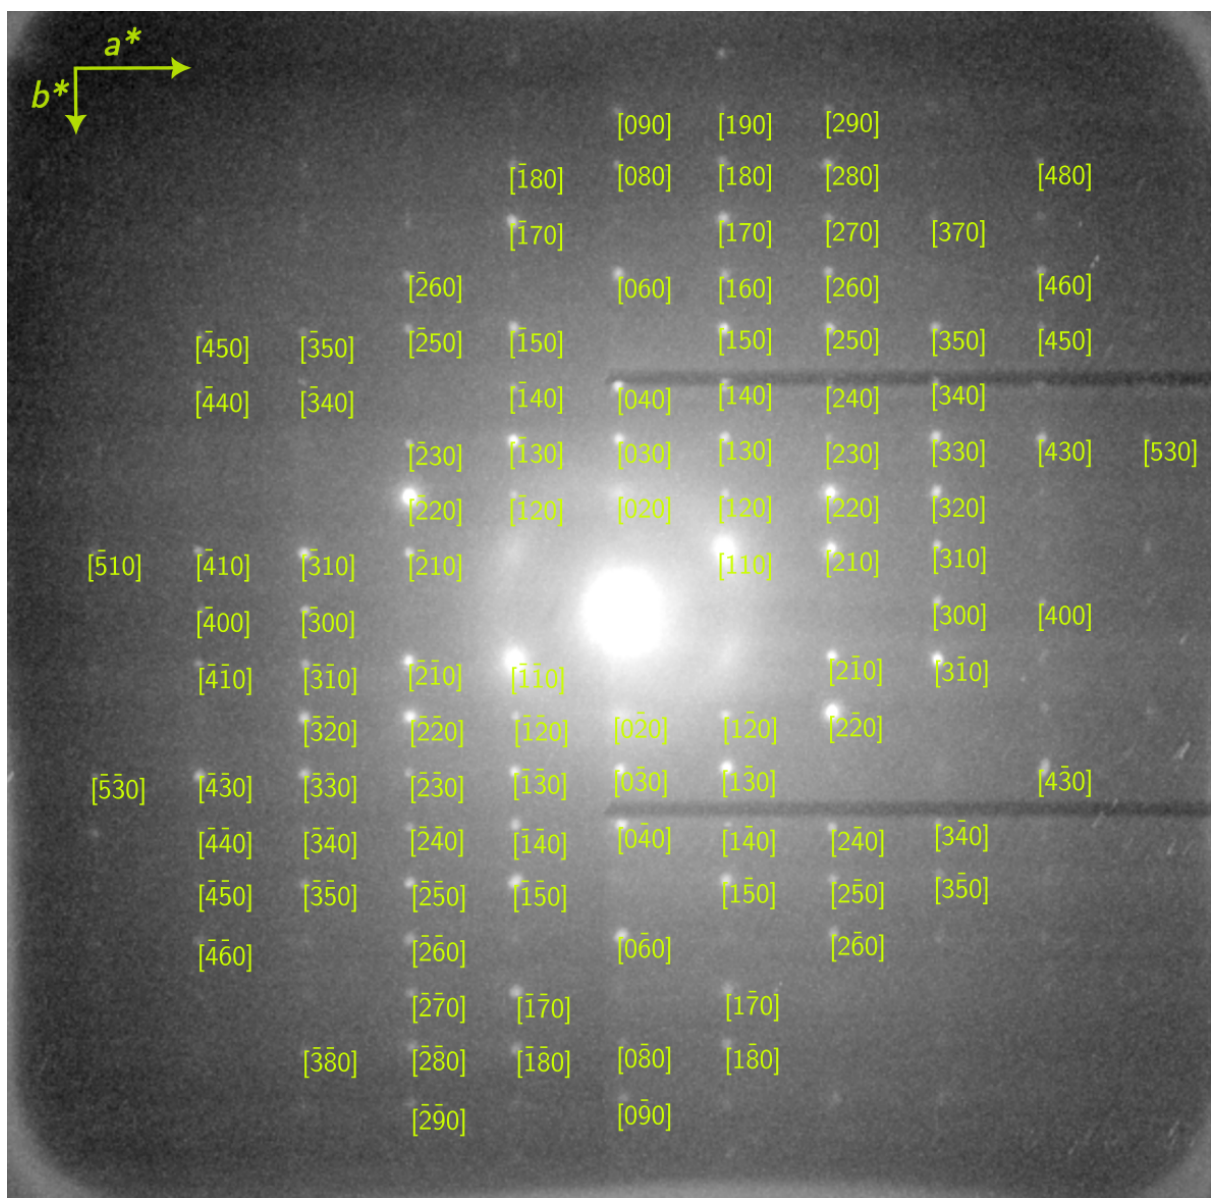

**Fig. S2.** Maximum diffraction pattern across all scans in the biotin time series, indexed by DIALS [47].

```
dxtbx.image_average -v *.img
dials.import max.cbf fast_slow_beam_centre=293,289 distance=136.5
dials.find_spots imported.expt threshold.algorithm=radial_profile blur=narrow
n_iqr=4 d_min=0.8
dials.index imported.expt strong.refl unit_cell="5.1955 10.3017 20.943 90 90
90" space_group=P212121 indexing.method=real_space_grid_search
crystal.fix=cell dials.image_viewer indexed.expt indexed.refl
```

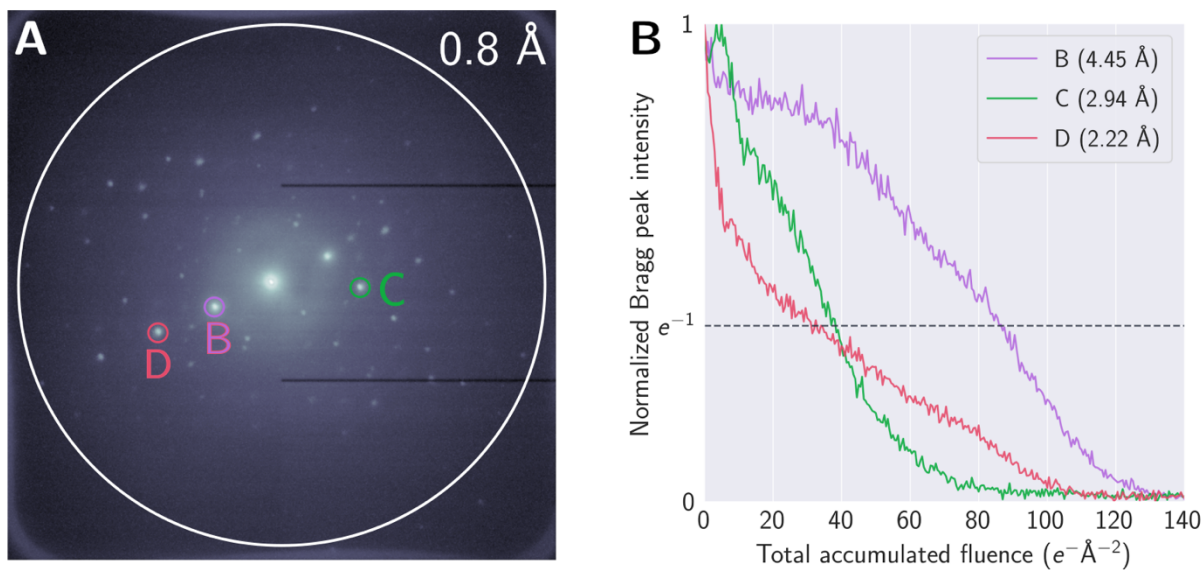

**Fig. S3. (A)** Maximum diffraction pattern across all scans in the Ni(dppf)Cl<sub>2</sub> time series, with virtual apertures (labeled B, C, and D) placed around the three progressively higher-resolution reflections referenced in Fig. 3 of the main text. **(B)** Decay profiles as a function of total accumulated fluence for each of the reflections encircled in **(A)**.

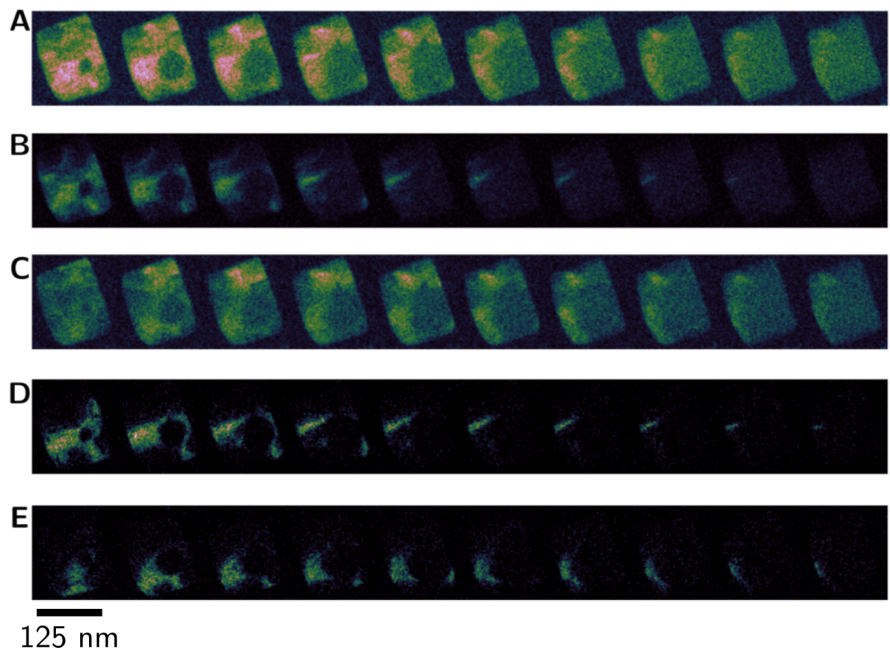

**Fig. S4.** VDF images visualizing the radial propagation of a tide of amorphization in Pd(dcy pf)Cl<sub>2</sub>, with a sampling interval of 5 4D-STEM scans per displayed image. (A) VDF images reconstructed by placing virtual apertures around 47 clearly identified Bragg peaks. (B) VDF images reconstructed by placing virtual apertures around all 17 clearly identified reflections which underwent monotonic decay. (C) VDF images reconstructed by placing virtual apertures around all 30 clearly identified reflections which underwent nonmonotonic decay. (D) VDF images reconstructed by placing a single virtual aperture around a weaker, higher-resolution Bragg peak. (E) VDF images reconstructed by placing a single virtual aperture around another weaker, higher-resolution Bragg peak.

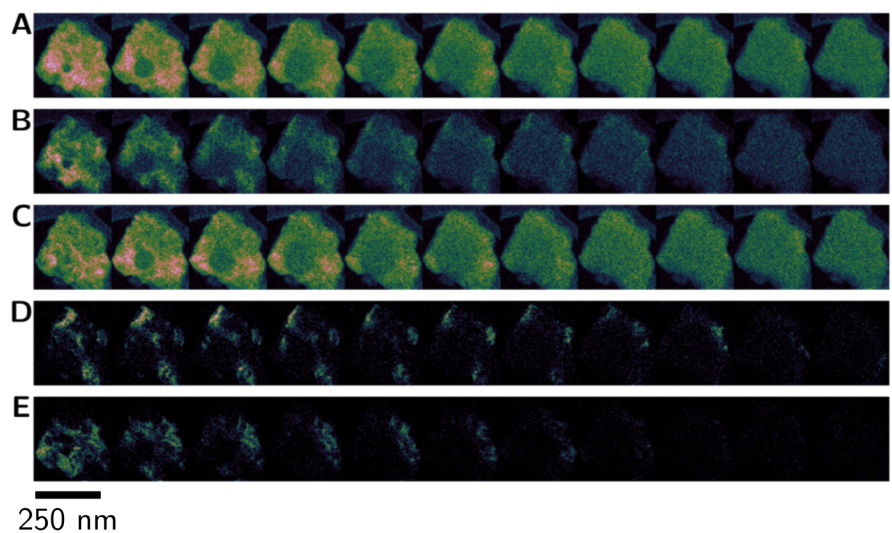

**Fig. S5.** VDF images visualizing the radial propagation of a tide of amorphization in  $\text{Pd(dppf)Cl}_2$ , with a sampling interval of 6 4D-STEM scans per displayed image. **(A)** VDF images reconstructed by placing virtual apertures around 45 clearly identified Bragg peaks. **(B)** VDF images reconstructed by placing virtual apertures around 14 clearly identified reflections which underwent monotonic decay. **(C)** VDF images reconstructed by placing virtual apertures around 31 clearly identified reflections which underwent nonmonotonic decay. **(D)** VDF images reconstructed by placing a single virtual aperture around a weaker, higher-resolution Bragg peak ( $d = 2.58 \text{ \AA}$ ). **(E)** VDF images reconstructed by placing a single virtual aperture around another weaker, higher-resolution Bragg peak ( $d = 1.75 \text{ \AA}$ ).

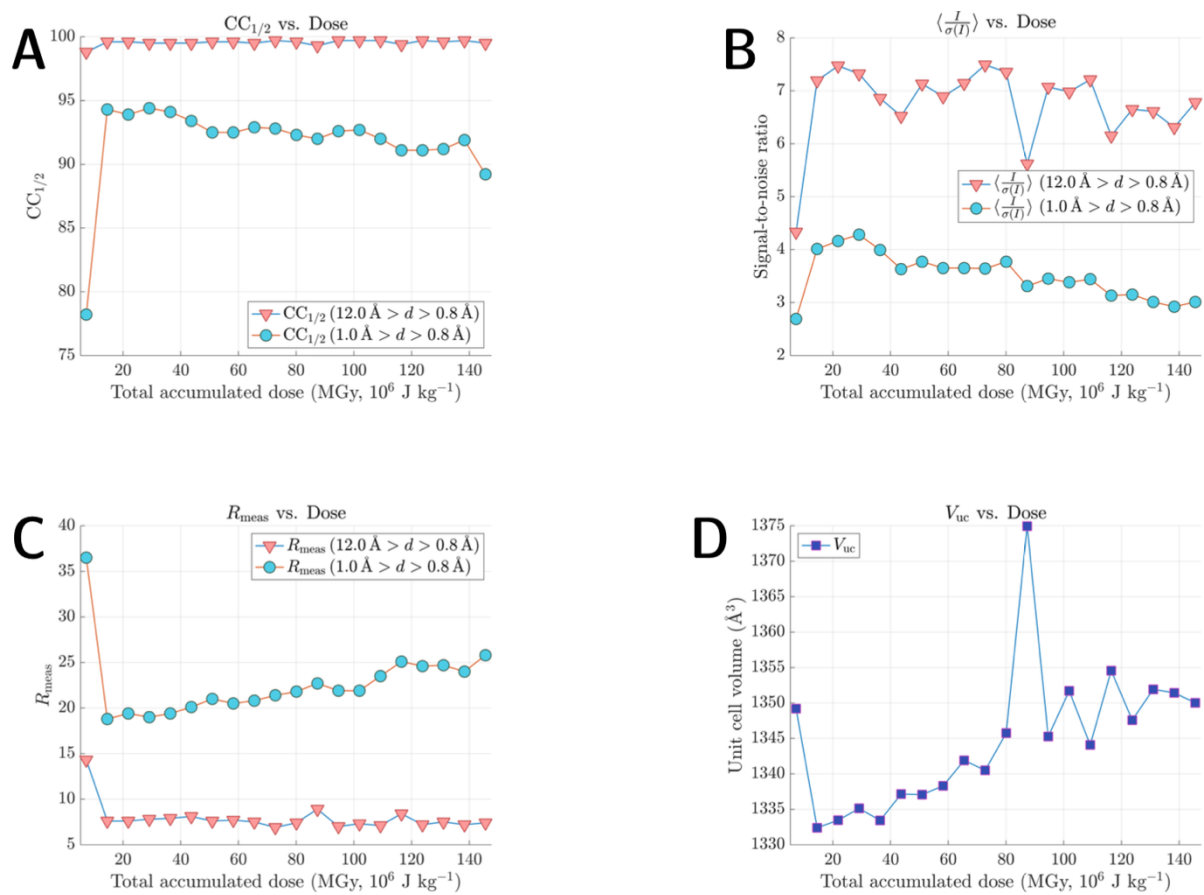

**Fig. S6.** Data reduction statistics for 20 consecutive 3D ED movies collected on a single crystal of  $\text{Ni(dppf)Cl}_2$ , where each point represents a full continuous-rotation dataset. A fluence of approximately  $2.2 \text{ e}^- \text{ \AA}^{-2}$  was delivered per movie, which was converted to a substrate-specific dose of 7.3 MGy using the program RADDose-EM [48]. After 20 consecutive passes, the  $\text{Ni(dppf)Cl}_2$  crystal has endured a total accumulated fluence of  $44 \text{ e}^- \text{ \AA}^{-2}$  (146 MGy). A clear improvement to a better value is seen between movies 1 and 2 for  $CC_{1/2}$  (**A**),  $\langle I/\sigma(I) \rangle$  (**B**), and  $R_{\text{meas}}$  (**C**), accompanied by a contraction in unit cell volume (**D**). From movie 2 onwards, all statistical metrics tend to uniformly get worse, and unit cell volume begins to expand. A plausible interpretation of these statistics is that data acquisition during the first movie is coterminous with significant CDZ reorientation, whereas the remainder of the movies represent the initial stages of slow, steady monotonic decay after the lattice has relaxed to a consensus orientation.

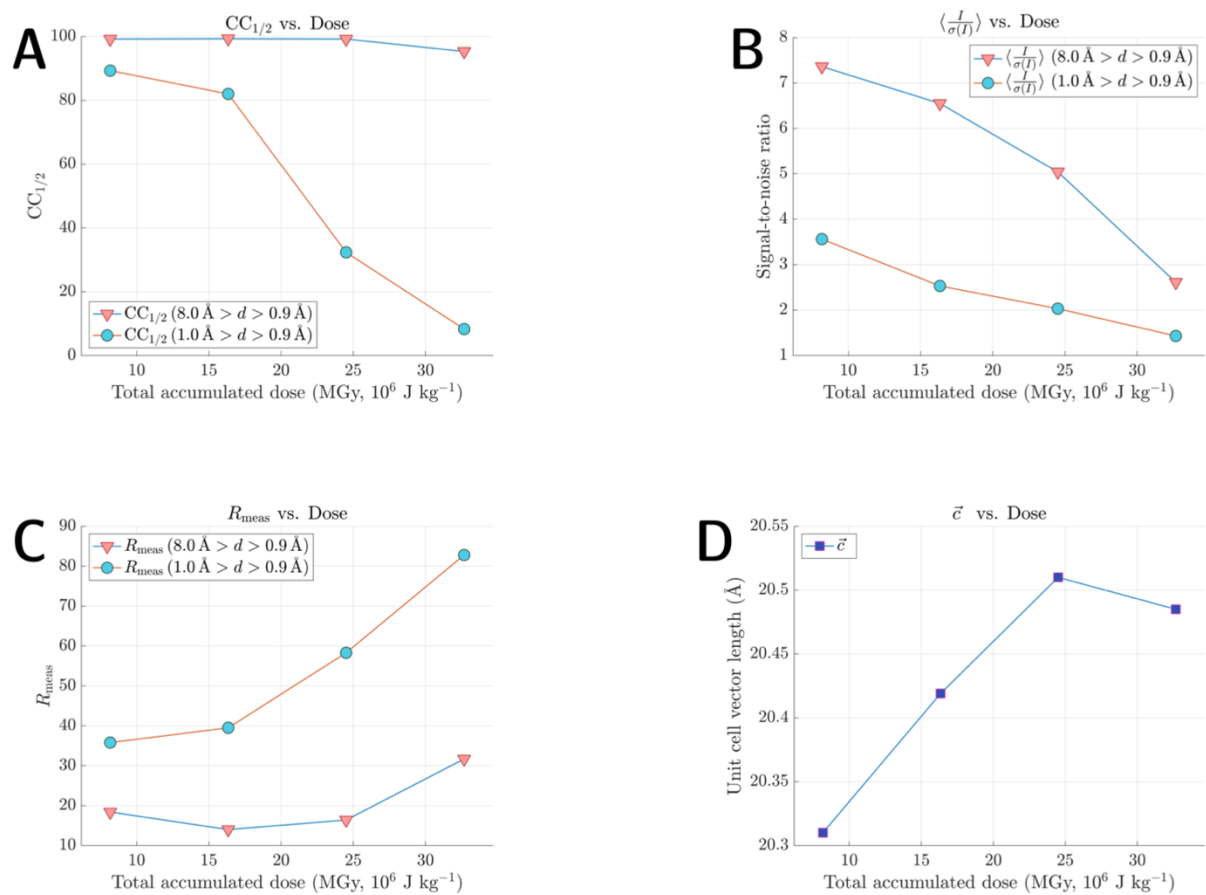

**Fig. S7.** Data reduction statistics for 4 consecutive 3D ED movies collected on a single crystal of biotin at 100 K, where each point represents a full continuous-rotation dataset. A fluence of approximately  $2.3 \text{ e}^- \text{ \AA}^{-2}$  was delivered per movie, which was converted to a substrate-specific dose of 8.2 MGy using the program RADDOS-EM [48]. After 20 consecutive passes, the biotin crystal has endured a total accumulated fluence of  $9.2 \text{ e}^- \text{ \AA}^{-2}$ , or 32.8 MGy. Unlike  $\text{Ni(dppf)Cl}_2$ , biotin is too beam-sensitive to allow acquisition of multiple 3D ED movies from the same crystal at RT, necessitating slow-cooling to cryogenic temperatures. Interestingly, these statistics appear mixed, with  $CC_{1/2}$  (**A**) and  $\langle I/\sigma(I) \rangle$  (**B**) deteriorating monotonically but overall  $R_{\text{meas}}$  (**C**) getting slightly better in movie 2. A plausible interpretation of these statistics is that CDZ reorientation has mostly concluded by the time movie 2 is acquired—thus the slightly better  $R_{\text{meas}}$ —but monotonic decay has also rapidly progressed to the point where  $CC_{1/2}$  (**A**) and  $\langle I/\sigma(I) \rangle$  have diminished, leading to overall lower-quality data.

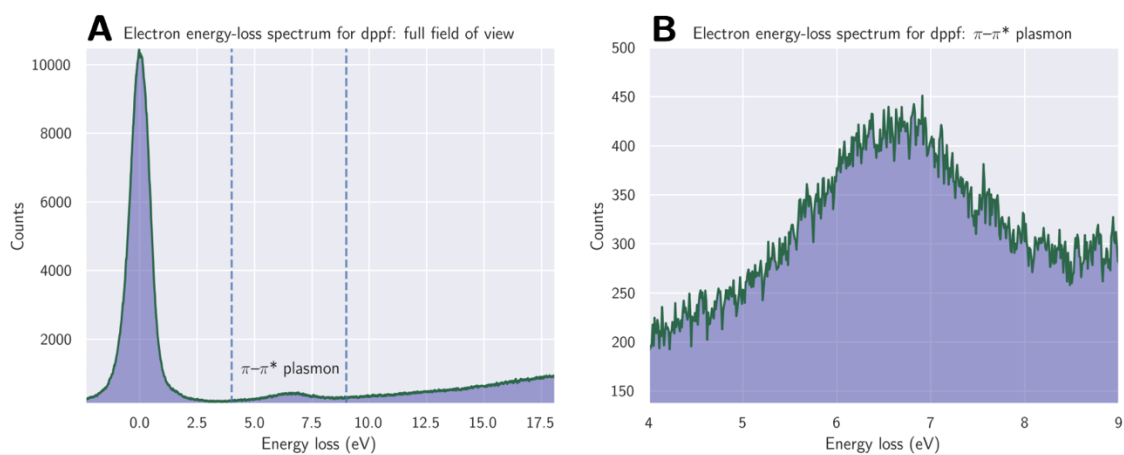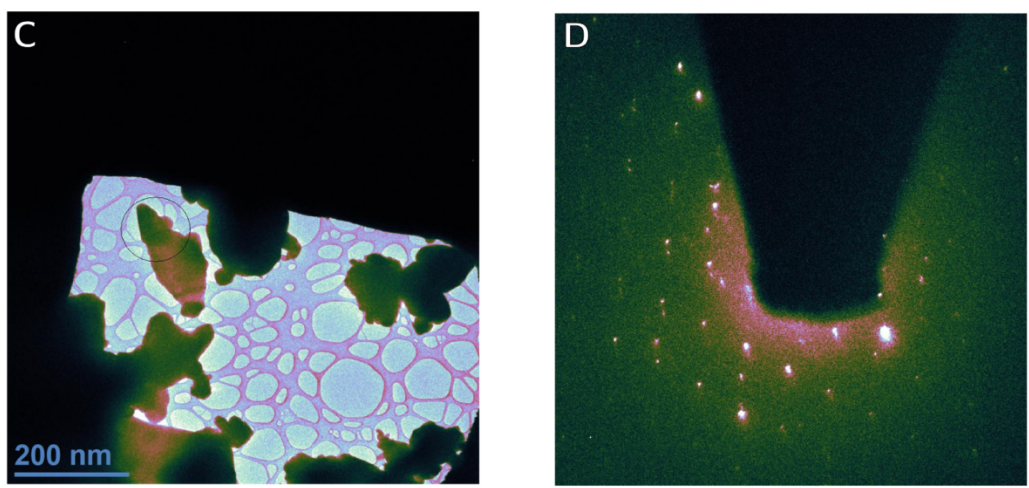

**Fig. S8.** Electron energy-loss spectrum (**A**, **B**) and selected-area diffraction pattern (**D**) acquired from a single crystal of dppf (**C**) before sustained irradiation.  $\pi-\pi^*$  plasmon is visible at 6.5 eV energy loss, with an estimated peak width of around 2.3 eV. Spectra were acquired using an FEI Tecnai F20 TEM equipped with a Gatan Imaging Filter (GIF) operating at an accelerating voltage of 200 kV.

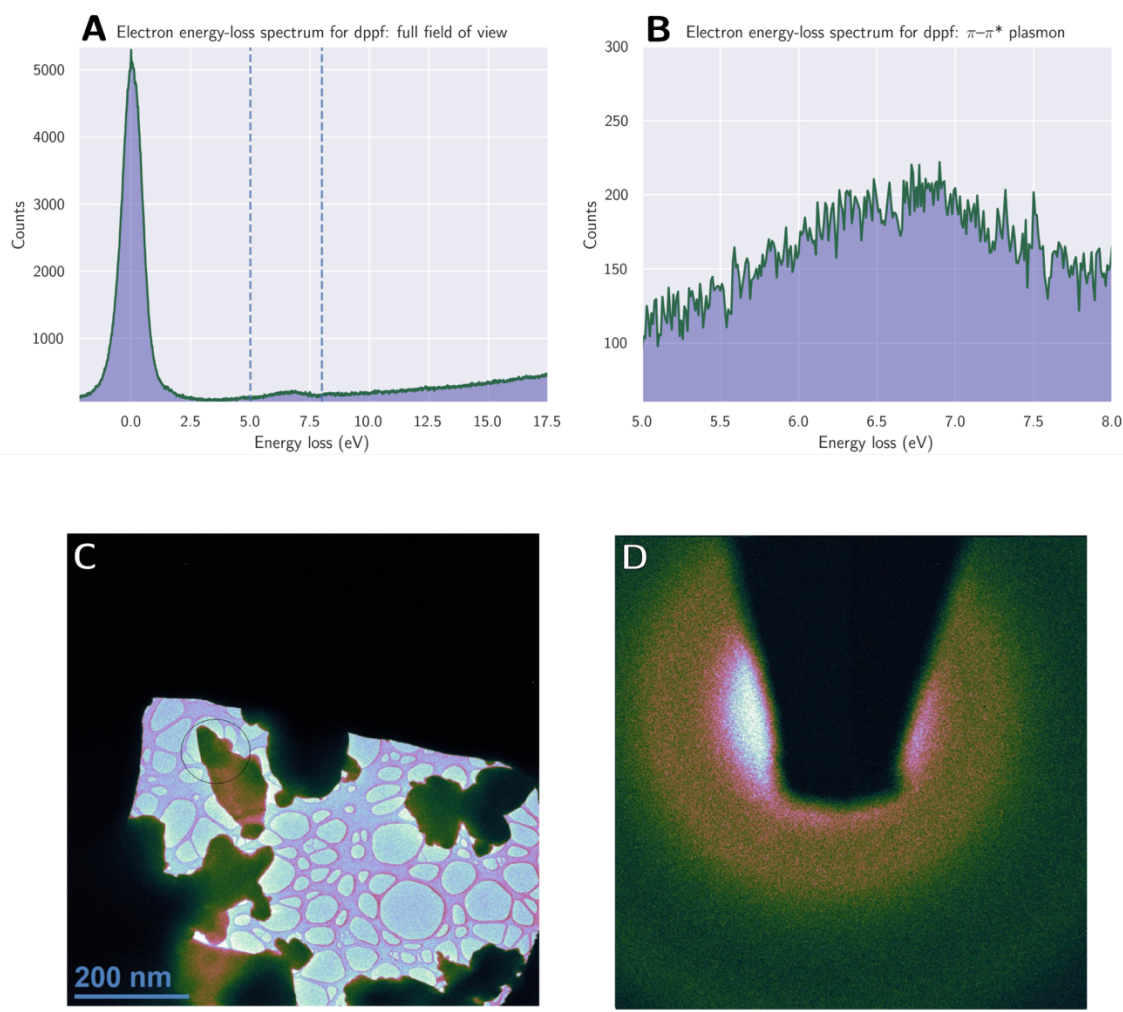

**Fig. S9.** Electron energy-loss spectrum (**A**, **B**) and selected-area diffraction pattern (**D**) acquired from a single crystal of dppf (**C**) after sustained irradiation for 10 minutes, corresponding to an estimated delivered fluence of  $300 \text{ e}^- \text{ \AA}^{-2}$ . Although the diffraction pattern has disappeared—indicating complete loss of crystallinity—the  $\pi$ - $\pi^*$  plasmon remains intact, indicating that crystallographic destruction precedes chemical destruction in this species. Interestingly, the  $\pi$ - $\pi^*$  peak is weaker and somewhat shifted compared to the pre-irradiation spectrum, now appearing at 6.3 eV energy loss with a

peak width of 2 eV. Spectra were acquired using an FEI Tecnai F20 TEM equipped with a Gatan Imaging Filter (GIF) operating at an accelerating voltage of 200 kV.

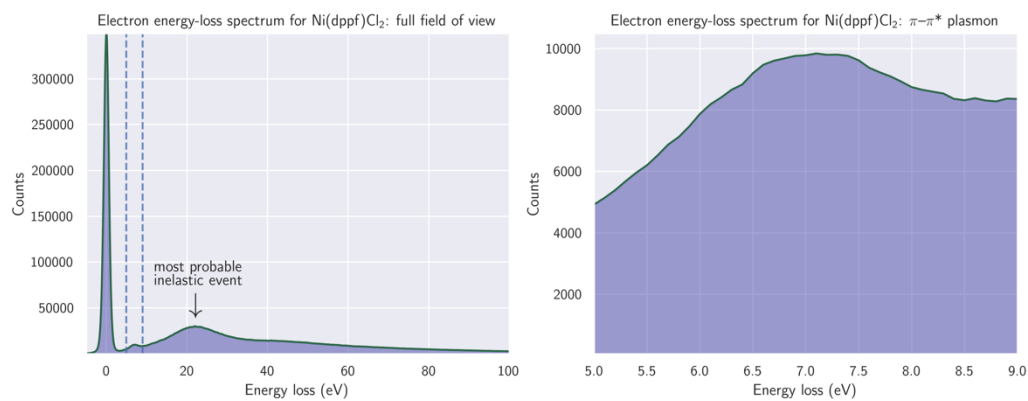

**Fig. S10.** Electron energy-loss spectrum acquired from a single crystal of Ni(dppf)Cl<sub>2</sub>, demonstrating that the most probable inelastic scattering event involves an energy loss of approximately 22 eV. Dashed vertical lines represent the  $\pi$ - $\pi^*$  plasmon corresponding to the presence of aromaticity. Spectra were acquired using a JEOL JEM-2100F TEM equipped with a Gatan Quantum SE operating at an accelerating voltage of 200 kV.
